# Supplementary material for: Differential Dynamic Programming for Nonlinear Dynamic Games
Source: arXiv:1809.08302 source file (2018-09-21)
Supplement: Supplementary file 1 [file appendix.tex]

\begin{lemma}
  \label{lem:newton_dp_solution}
  The solution to problem \ref{problem:auxiliary_dynamic} via dynamic programming has the following form

        State-action cost-to-go functions
        \begin{align}
          sf
            \label{eq:newton_dp_solution_state_action_val_fun}
            Q_{n,k}(\delta x_k, \Delta x_k, \delta u_{:,k}) = \frac{1}{2} \left(
            \begin{bmatrix}
            %   1 \\
            %   \delta x_k \\
            %   \delta u_{:,k}
            % \end{bmatrix}^T \Gamma_{n,k}
            % \begin{bmatrix}
            %   1 \\
            %   \delta x_k \\
            %   \delta u_{:,k}
            % \end{bmatrix} + \Omega_{n,k} \Delta x_k \right)
          \end{align}

    \begin{align}
      V_{n,k}(\delta x_k, \Delta x_k) = \frac{1}{2} \left(
      \begin{bmatrix}
        1 \\
        \delta x_k
      \end{bmatrix}^T S_{n,k}
        \begin{bmatrix}
          1 \\
          \delta x_k
        \end{bmatrix} + \Omega_{n,k} \Delta x_k \right)
    \end{align}
    Equilibrium affine policy
    \begin{align}
      \label{eq:newton_dp_minimizer}
      \delta u_{:,k} = K_k \delta x_k + s_k
    \end{align}
  \end{subequations}
  where the matrices are found
  \begin{subequations}
    \label{eq:newton_dp_matrices}
    \begin{align}
      & \Gamma_{n,T} = M_{n,T} \\
      & \Gamma_{n, k} =
      \begin{bmatrix}
        \Gamma_{n, k}^{11} & \Gamma_{n, k}^{1x} & \Gamma_{n, k}^{1u} \\
        \Gamma_{n, k}^{x1} & \Gamma_{n, k}^{xx} & \Gamma_{n, k}^{xu} \\
        \Gamma_{n, k}^{u1} & \Gamma_{n, k}^{ux} & \Gamma_{n, k}^{uu}
      \end{bmatrix} \nonumber \\
      & \quad \ =
      \begin{bmatrix}
        \Gamma_{n, k}^{11} & \Gamma_{n, k}^{1x} & \Gamma_{n, k}^{1u_1} & \Gamma_{n, k}^{1u_2} & \cdots & \Gamma_{n, k}^{1u_N} \\
        \Gamma_{n, k}^{x1} & \Gamma_{n, k}^{xx} & \Gamma_{n, k}^{xu_1} & \Gamma_{n, k}^{xu_2} & \cdots & \Gamma_{n, k}^{xu_N} \\
        \Gamma_{n, k}^{u_11} & \Gamma_{n, k}^{u_1x} & \Gamma_{n, k}^{u_1u_1} & \Gamma_{n, k}^{u_1u_2} & \cdots & \Gamma_{n, k}^{u_1u_N} \\
        \Gamma_{n, k}^{u_21} & \Gamma_{n, k}^{u_2x} & \Gamma_{n, k}^{u_2u_1} & \Gamma_{n, k}^{u_2u_2} & \cdots & \Gamma_{n, k}^{u_2u_N} \\
        \vdots & \vdots & \vdots & \vdots & \ddots & \vdots \\
        \Gamma_{n, k}^{u_N1} & \Gamma_{n, k}^{u_Nx} & \Gamma_{n, k}^{u_Nu_1} & \Gamma_{n, k}^{u_Nu_2} & \cdots & \Gamma_{n, k}^{u_Nu_N}
      \end{bmatrix} \\
      & F_k =
      \begin{bmatrix}
        \Gamma_{1k}^{u_1u} \\
        \Gamma_{2k}^{u_2u} \\
        \vdots \\
        \Gamma_{Nk}^{u_Nu}
      \end{bmatrix} =
      \begin{bmatrix}
        \Gamma_{1k}^{u_1u_1} & \Gamma_{1k}^{u_1u_2} & \cdots & \Gamma_{1k}^{u_1u_N} \\
        \Gamma_{2k}^{u_2u_1} & \Gamma_{2k}^{u_2u_2} & \cdots & \Gamma_{2k}^{u_2u_N} \\
        \vdots & \vdots & \ddots & \vdots \\
        \Gamma_{Nk}^{u_Nu_1} & \Gamma_{Nk}^{u_Nu_2} & \cdots & \Gamma_{Nk}^{u_Nu_N}
      \end{bmatrix} \\
      & P_k =
      \begin{bmatrix}
        \Gamma_{1k}^{u_1x} \\
        \Gamma_{2k}^{u_2x} \\
        \vdots \\
        \Gamma_{Nk}^{u_Nx}
      \end{bmatrix}, \quad
      H_k =
      \begin{bmatrix}
        \Gamma_{1k}^{u_11} \\
        \Gamma_{2k}^{u_21} \\
        \vdots \\
        \Gamma_{Nk}^{u_N1}
      \end{bmatrix} \\
      & s_k = - F_k^{-1} H_k, \quad K_k = - F_k^{-1} P_k \\
      \label{eq:newton_dp_solution_S}
      & S_{n, k} =
      \begin{bmatrix}
        1 & 0 & 0 \\
        0 & I & K_k^\top
      \end{bmatrix} \Gamma_{n, k}
      \begin{bmatrix}
        1 & 0 \\
        0 & I \\
        0 & K_k
      \end{bmatrix} \nonumber \\
      & \quad \ +
      \begin{bmatrix}
        s_k^\top \Gamma_{n, k}^{uu} s_k + 2 s_k^\top \Gamma_{n, k}^{u1} & s_k^\top (\Gamma_{n, k}^{ux} + \Gamma_{n, k}^{uu} K_k) \\
        (\Gamma_{n, k}^{ux} + \Gamma_{n, k}^{uu} K_k)^\top s_k & 0
      \end{bmatrix} \\
      \label{eq:GammaDef}
      & \Gamma_{n,k} = M_{n,k} \nonumber \\
      & +
      \begin{bmatrix}
        S_{n, k+1}^{11} & S_{n,k+1}^{1x}A_k & S_{n,k+1}^{1x}B_k \\
        A_k^\top S_{n,k+1}^{x1} & A_k^\top S_{n,k+1}^{xx}A_k + D_k^{xx} & A_k^\top S_{n,k+1}^{xx} B_k + D_k^{xu} \\
        B_k^\top  S_{n,k+1}^{x1}  & B_k^\top  S_{n,k+1}^{xx}A_k + D_k^{ux} & B_k^\top S_{n,k+1}^{xx} B_k + D_k^{uu}
      \end{bmatrix} \\
      \label{eq:newton_dp_solution_omega0}
      & \Omega_{n,T} = M_{n,T}^{1x} \\
      \label{eq:newton_dp_solution_omega1}
      & \Omega_{n,k} = M_{n,k}^{1x} + \Omega_{n,k+1} A_k \\
      \label{eq:newton_dp_solution_D}
      & D_{n,k} = \sum_{l=1}^n \Omega_{n,k+1}^l G_k^l
    \end{align}
  \end{subequations}
  and $n = 1, 2, \ldots, N$ and $k = 0, 1, \ldots, T$.
\end{lemma}

%%% Local Variables:
%%% mode: latex
%%% TeX-master: di2019differential
%%% End:
